# Supplementary material for: Linked Adapters: Linking Past and Future to Present for Effective Continual Learning
Source: arXiv:2412.10687 source file (2024-12-14)
Supplement: Supplementary file 1 [file X_suppl.tex]

\clearpage
\setcounter{page}{1}
\maketitlesupplementary

\section{Experiments}

\subsection{Architectural details}
For experiments in Table~\ref{table:1}, We chose pre-trained ViT\_B\_16 as our base model where it has approximately 86M parameters, which comprises 12 layers. For approaches that employ adapters, it is incorporated between the multi-headed self-attention (MHSA) and feed-forward layers (FFN) at every layer of the transformer. Hidden state input to adapter is 768 dimension from MHSA. Subsequently, we downsample this to 96 dimensions before upsampling it back to 768 dimensions, which is then fed into the FFN. Adding adapters at every layer of transformer grows approximately 2\% parameters per task compared to  ViT\_B\_16. This growth in parameters is same across the experiments on standalone adapters and Linked adapters. To generate attention weights between task \textit{p} and task \textit{t}, MLP takes concatenated input of task specific embeddings ($\mathbf{e}^p$,$\mathbf{e}^t$), each of size 32 dimensions.
The MLP responsible for generating attention weights consists of three fully connected layers. It takes a 64-dimensional input, which is the concatenation of the embeddings, and produces a 12-dimensional output representing the attention weights from task \textit{p} to task \textit{t} at every layer of transformer. The architecture of the MLP can be described as a series of three fully connected layers with dimensions 64*32, 32*16, and 16*12. To reproduce the results reported in Table~\ref{table:1}, we randomly initialised weights of adapters and MLP with seed. In addition, to mitigate the risk of forgetting during the training of the MLP when adapting to new tasks, the regularization constant $\lambda$ is chosen based on the validation dataset. In the reported results for the Cifar datasets in Table~\ref{table:1}, a learning rate of 0.1 is utilised, while for the Cub200 dataset, a learning rate of 0.3 is utilised. Our experiments utilized a single NVIDIA Tesla V100 GPU. The CIFAR-10/CIFAR-100 dataset with different splits required around 30 minutes training time, while the Cub-200 dataset took approximately 10 minutes training time.

\subsection{Task Ordering }
In our experiments on the CUB-200 dataset with 5-splits, we evaluated the knowledge transfer capabilities of our proposed models, Adalink-forward and Adalink-bidirectional, under varying task orders. Unlike traditional experiments where tasks are presented in a fixed order, we intentionally introduced randomized task sequences to demonstrate effectiveness of proposed approaches in knowledge transfer across tasks irrespective of task order. In the paradigm of learning independent adapters for each task, the learning process remains unaffected by the ordering of tasks. However, our proposed approaches, Adalink-Forward and Adalink-Bidirectional, maintains connections with other task, task ordering could affect the performance. In Table~\ref{table:randomorders}, 5-splits of Cub200 are presented in random orders(RO1,RO2,RO3,RO4) and accuracies of AdaLink-forward and AdaLink-bidirectional are reported in respective orders. In Figure~\ref{fig:random_orders} , both AdaLink-forward and AdaLink-bidirectional consistently demonstrated robust knowledge transfer, showcasing their resilience to changes in task order. AdaLink-forward effectively utilized lateral connections to transfer knowledge from previous tasks to the current one. The forward attention weights, generated by the MLP, seamlessly adjusted to different task orders, ensuring the selective retention of information across the entire task sequence. AdaLink-bidirectional consistently outperforms standalone adapters and AdaLink-forward in all task orders, as depicted in Figure \ref{fig:random_orders}.
\begin{figure}
  \centering
  \includegraphics[width=1\linewidth, height=8cm]{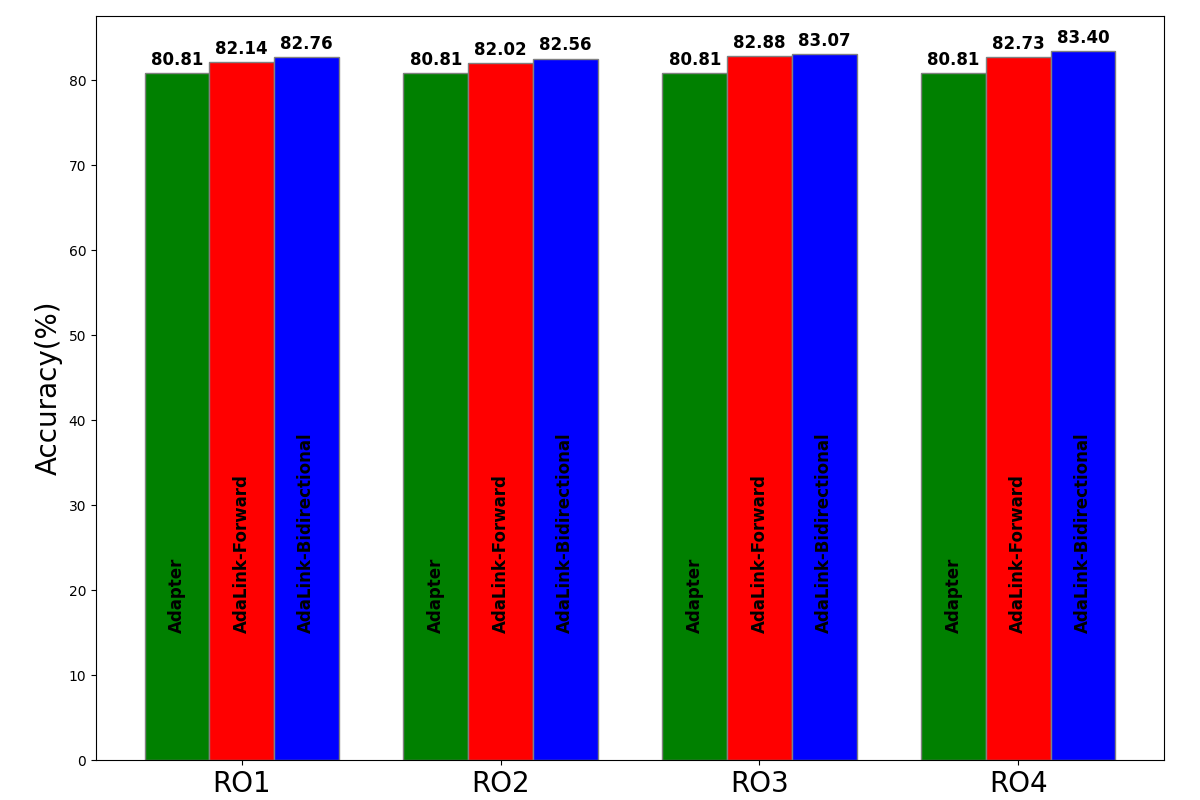}
  \caption{Comparison of average test accuracies of Adapter, AdaLink-Forward, AdaLink-Bidirectional over 4 different random orders (RO1,RO2,RO3,RO4).}
  \label{fig:random_orders}
\end{figure}

\begin{table}
    \centering
   {
        \begin{tabular}{|c|c|c|}
            \hline
            {Task Order } &{AdaLink-Forward}&{AdaLink-Bidirectional} \\
            \hline
            RO1- 41230 & 82.14 $\pm$ 0.69 & 82.76 $\pm$ 0.44\\
            \hline
            RO2- 43210 & 82.02 $\pm$ 1.40 & 82.56 $\pm$ 0.98\\
            \hline
            RO3- 21403& 82.88 $\pm$ 0.98& 83.07 $\pm$ 0.81\\
            \hline
            RO4- 01423& 82.73 $\pm$ 0.95 & 83.40 $\pm$ 0.75\\
             \hline
        \end{tabular}
    }
    \caption{Average test accuracies of AdaLink-Forward, AdaLink-Bidirectional over 4 different random task orders}
    \label{table:randomorders}
\end{table}

\subsection{Backward Transfer}
 To validate the effectiveness of \textit{AdaLink-Bidirectional} in enabling Backward Transfer over sequence of tasks, we compute a \textit{Backward Transfer(BT)} metric. The average backward transfer across all the tasks can be computed as $BT=\frac{1}{m}\sum_{i=1}^{m} {acc}_{end,i} - {acc}_{during,i}$. Here, ${acc}_{end,i}$ represents the accuracy achieved on the $i^{th}$ task when using \textit{AdaLink-Bidirectional} after training on all tasks, and ${acc}_{during,i}$ denotes the accuracy on the $i^{th}$ task when trained and tested after the $i^{th}$ task in the sequential order.

 The reported average backward transfer of 0.35\% on Cub 200 5-splits and 0.38\% on Cub 200 with 10-splits showcase the capability of the proposed \textit{AdaLink-Bidirectional} approach in transferring knowledge in the backward direction, as detailed in Table \ref{tab:back}. The individual task accuracies of \textit{AdaLink} during training are computed by evaluating accuracy for each task after its dedicated training phase. Figure~\ref{fig:back} (a) demonstrate backward transfer of \textit{AdaLink-Bidirectional} compared to \textit{AdaLink} during training on Cub200 with 5 splits and Figure~\ref{fig:back} (b) on Cub200 with 10 splits.

\begin{table}
    \centering
   {
        \begin{tabular}{|c|c|}
            \hline
            \textbf{Cub200 } & \textbf{BT(\%)} \\
            \hline
            5 Splits & 0.35\\
            \hline
            10 Splits & 0.38 \\
            \hline
        \end{tabular}
    }
    \caption{Average backward transfer(BT) on Cub200 dataset with 5-Splits and 10-Splits}
    \label{tab:back}
\end{table}

 \begin{figure*}
    \centering
    
    \begin{subfigure}{0.49\textwidth}
        \includegraphics[width=\linewidth]{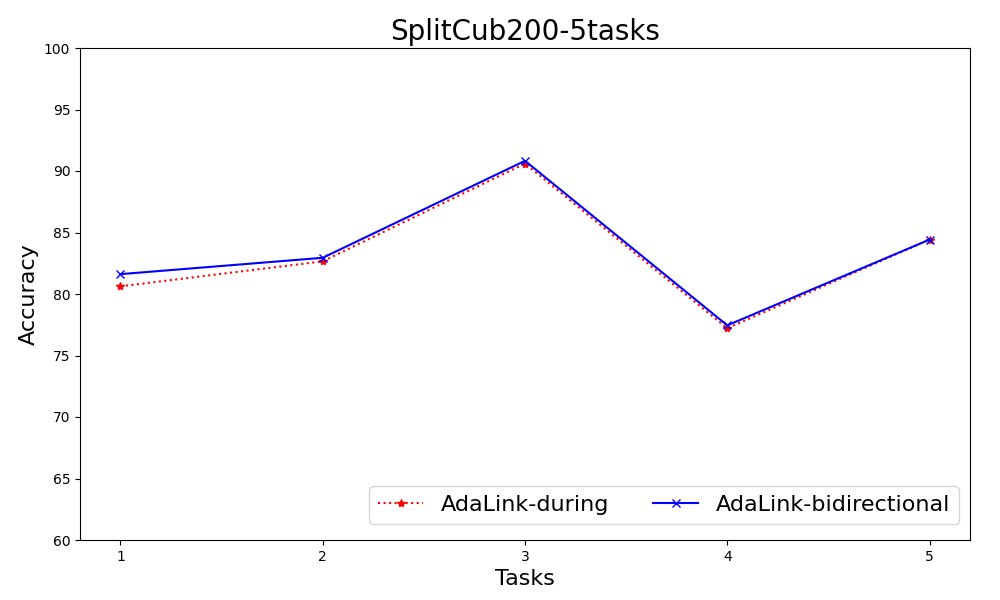}
        \caption{}
        \label{fig:sub1}
    \end{subfigure}
    \hfill
    \begin{subfigure}{0.49\textwidth}
        \includegraphics[width=\linewidth]{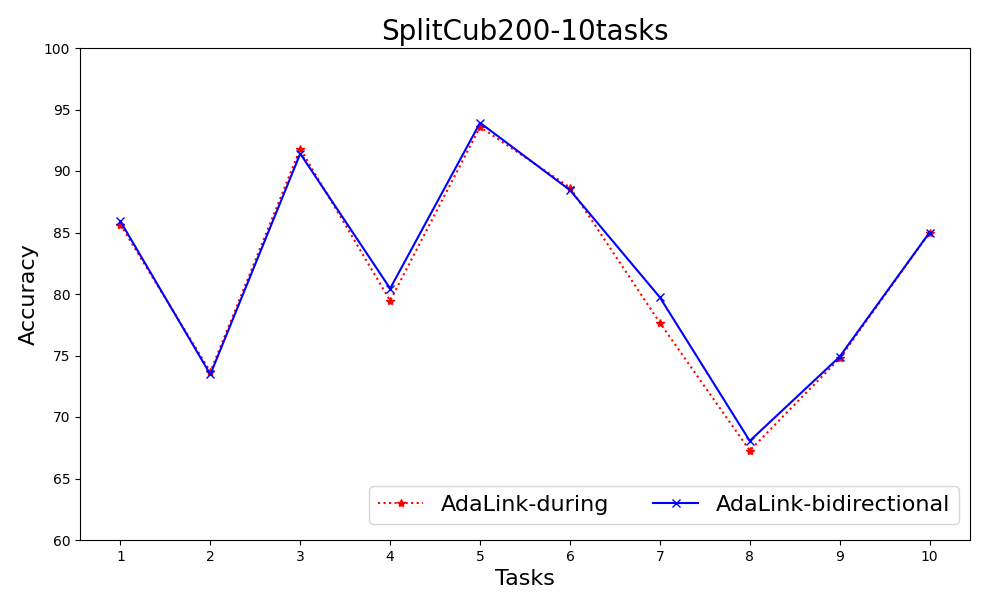}
        \caption{}
        \label{fig:sub2}
    \end{subfigure}
      \caption{Comparing indvidiual task accuracy(\%): AdaLink during Training vs. AdaLink Bidirectional. Here, AdaLink during Training refers computing accuracy for task after its dedicated training phase. In the above figure, on X-axis tasks numbers are mentioned and on Y-axis, average test accuracy of individual tasks are presented }
    \label{fig:back}
\end{figure*}

\begin{figure*}
    \centering
    
    \begin{subfigure}{0.49\textwidth}
        \includegraphics[width=\linewidth]{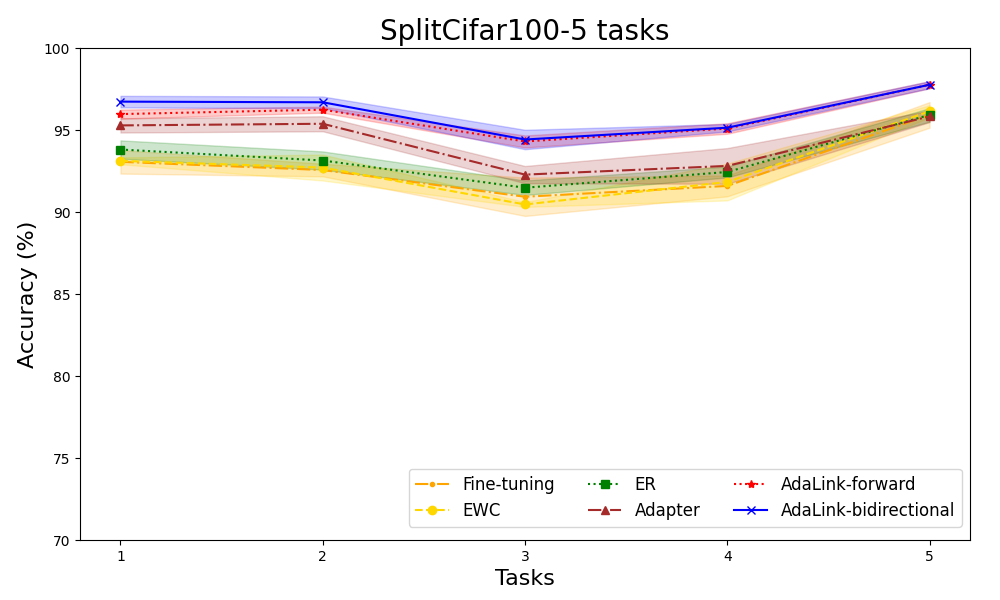}
        \caption{}
        \label{fig:sub1}
    \end{subfigure}
    \hfill
    \begin{subfigure}{0.49\textwidth}
        \includegraphics[width=\linewidth]{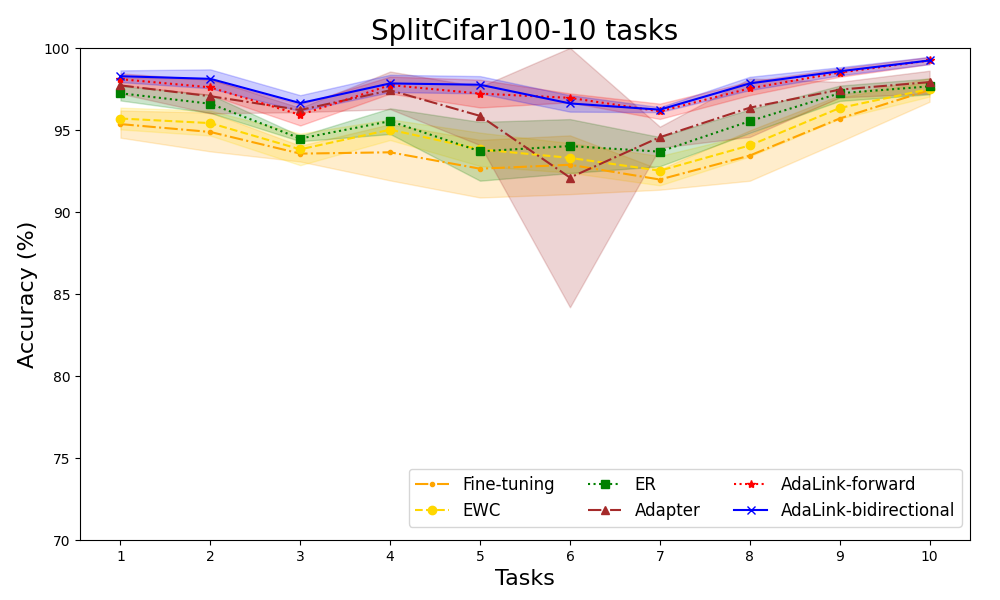}
        \caption{}
        \label{fig:sub2}
    \end{subfigure}
    
    \vspace{1em}
    
    \begin{subfigure}{0.49\textwidth}
        \includegraphics[width=\linewidth]{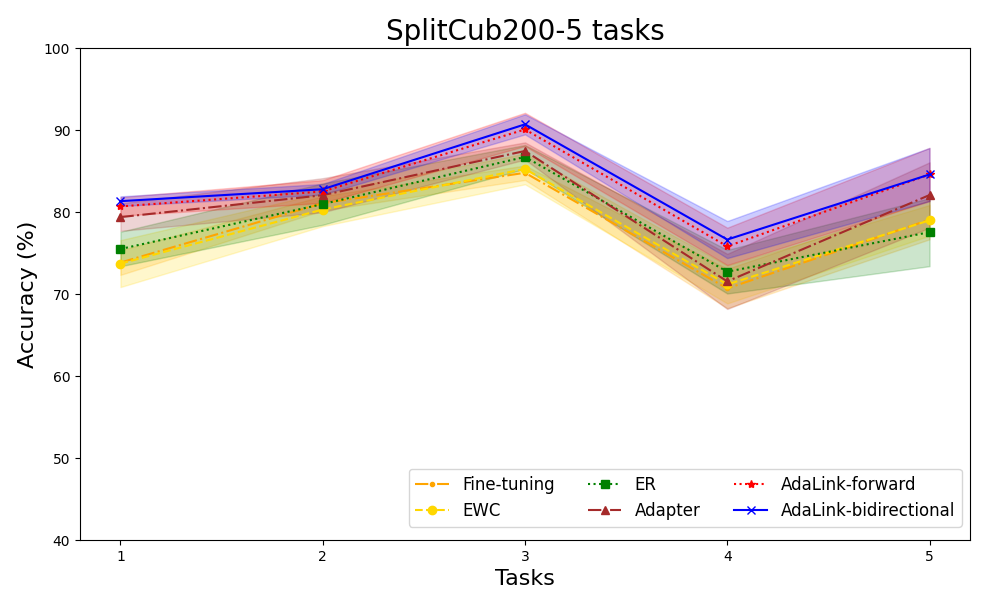}
        \caption{}
        \label{fig:sub3}
    \end{subfigure}
    \hfill
    \begin{subfigure}{0.49\textwidth}
        \includegraphics[width=\linewidth]{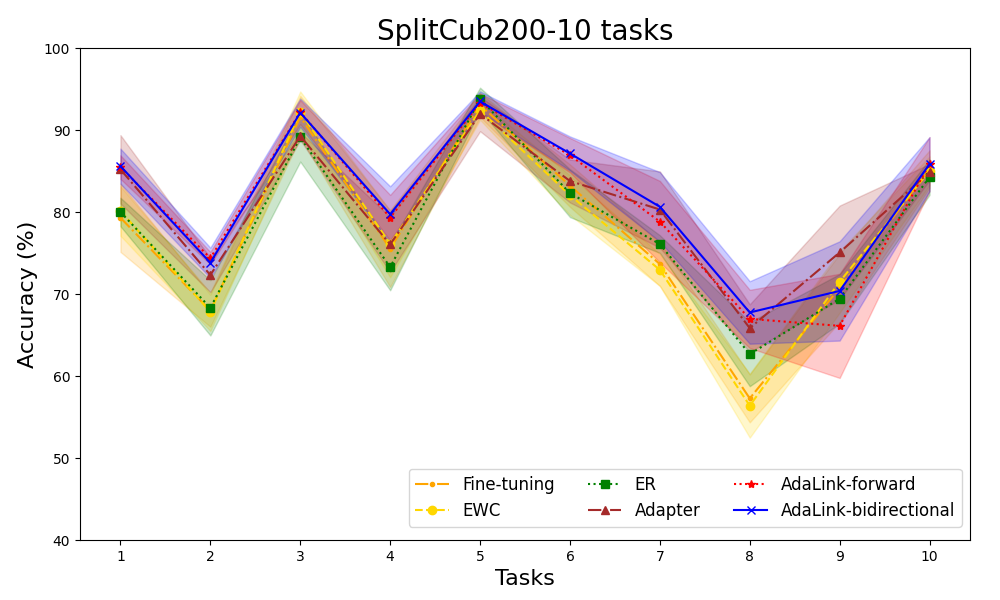}
        \caption{}
        \label{fig:sub4}
    \end{subfigure}

    \caption{ Comparison between baselines and \textit{AdaLink} over average test accuracy of individual tasks. In the above figure, on X-axis tasks numbers are mentioned and on Y-axis, average test accuracy of individual tasks are presented (computed over 5 random seed initialisation) }
    \label{fig:overall_std}
\end{figure*}
\subsection{Performance Variance}
We also plotted results of  baselines and AdaLink over average test accuracy of individual tasks. In Figure~\ref{fig:overall_std}, individual task accuracy with standard deviation over 5 random seeds are plotted. Figure~\ref{fig:overall_std} (a) demonstrates the effectiveness of AdaLink-Bidirectional over all the baselines on SplitCifar100 5-splits and  Figure~\ref{fig:overall_std} (b) on SplitCifar100 10-splits. Similarly, Figure~\ref{fig:overall_std} (c) and Figure~\ref{fig:overall_std} (d)  demonstrates the effectiveness of AdaLink-Bidirectional over all the baselines on SplitCub200 5-splits and 10-splits respectively.
